# Supplementary material for: Pressure-tuned many-body phases through $\Gamma$-K valleytronics in moir\'e bilayer WSe$_2$
Source: arXiv:2404.07165 source file (2024-04-10)
Supplement: Supplementary file 1 [file WSe2_SupplInfo.pdf]

# Supplementary Information for:
# Pressure-tuned many-body phases through Γ-K valleytronics in moiré bilayer $WSe_2$

Marta Brzezińska, Sergii Grytsiuk, Malte Rösner, Marco Gibertini, and Louk Rademaker

(Dated: April 10, 2024)

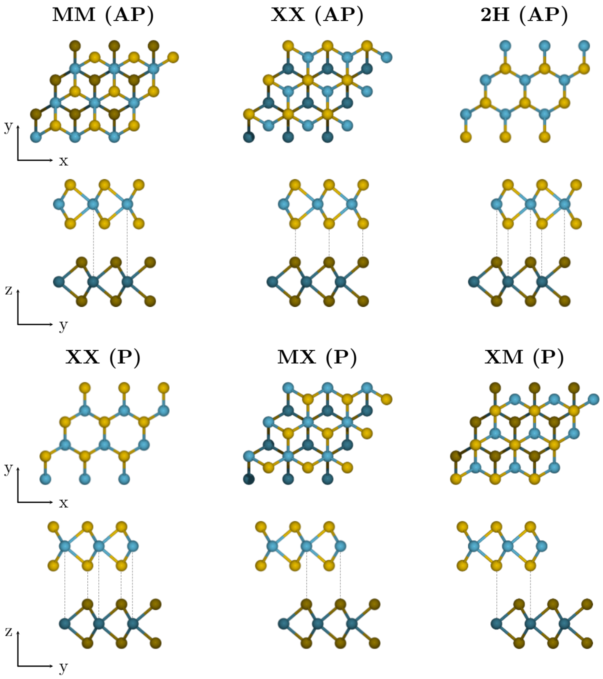


FIG. 1. Top and side views of six commensurate stackings $WSe_2$ bilayers. Blue color corresponds to the W atoms, while yellow to the Se atoms. The atoms from the bottom layer are represented in a darker shade.

# I. DENSITY FUNCTIONAL THEORY CALCULATIONS

Density functional theory (DFT) calculations were done using QUANTUM ESPRESSO [1–3] and fully relativistic norm-conserving pseudopotentials from PseudoDojo suite [4]. We performed convergence tests for a parallel XX configuration and carried over the computational parameters to the remaining structures. To achieve a total energy convergence within 1 meV/atom, we set the plane wave cutoff to 90 Ry (and thus the charge density cutoff to 360 Ry) and use a $12 \times 12 \times 1$ $\Gamma$-centered Monkhorst-Pack **k**-grid. Spurious interactions with artificial periodic replicas are removed by using a Coulomb cutoff technique [5, 6]. For structural relaxations, we employed the BFGS algorithm and set the convergence threshold on forces for ionic minimization to be 2.6 meV/Å and included the effect of van der Waals (vdW) interactions using the rVV10 functional [7, 8] in a non-relativistic framework. DFT data processing was done with the ASE package [9].

### A. Description of the high-symmetry stackings

TMD homobilayers can be produced, for instance, by 'tear and stack' fabrication technique, where the layers are either arranged in *parallel* (P, if a rotation angle between the layers is $\theta \sim 0°$) or *antiparallel* configuration (AP, $\theta \sim 180°$) [cf. Fig. 1]. These stacking orders resemble the 3R (rhombohedral) and 2H (trigonal) phases of bulk crystal, respectively. Due to atomic reconstruction, the moiré lattices exhibit locally high-symmetry stackings. For parallel configurations, we can distinguish three commensurate stackings: XX (also called AA), where metal and chalcogenide atoms from both layers are aligned along $z$-axis, and MX (XM), where metal (chalcogenide) atom from a top layer is aligned with chalcogenides (metals) from a bottom layer. MX and XM stackings are related to each other by a mirror symmetry. For antiparallel configurations, there are MM (metal over metal), XX (chalcogenide over chalcogenide), and 2H (all atoms are aligned) stackings. 2H posseses an inversion symmetry.

### B. Comparisons of different functionals

Layered materials are not correctly described by (semi)-local functionals as they do not capture a long-range nature of vdW interactions. Here, we systematically study several commonly used correction schemes with a parallel XM configuration at experimental in-plane lattice constant $a = 3.288$ Å [10] as an example. We relaxed the structure within a fixed cell geometry, allowing only the atomic positions to change. As most of the non-local vdW functionals have not been developed to include non-collinear effects yet, we relaxed the structure without spin-orbit coupling (SOC) using norm-conserving scalar-relativistic pseudopotentials from PseudoDojo [4]. Self-consistent and band structure calculations are then performed for the optimized geometry with the standard PBE functional and including SOC. For empirical corrections, SOC was included at all steps of calculations. The results for dispersion-corrected PBE functionals [11–14] and vdW functionals [7, 8, 15–23] are listed in Table I. Depending on the vdW corrections, the resulting optimal equilibrium distance can vary significantly, up to 0.5 Å. As expected, pure PBE functional overestimates $d_0$, followed by the vdW-DF family of functionals. We recall that the interlayer spacing of bulk $WSe_2$ is 6.51 Å [24], although it corresponds to a different stacking (AP XM, i.e. 2H).

|  | $d_0$ (Å) | $\Delta E$ (eV) | $\Delta_{\Gamma K}$ (meV) | $\Delta_{\Gamma_0 \Gamma_{-1}}$ (meV) |
|---|---|---|---|---|
| PBE | 7.800 | 1.195 | -475.3 | 199.2 |
| Grimme-D2 | 6.462 | 1.077 | -89.4 | 681.9 |
| Grimme-D3 | 6.624 | 1.090 | -178.3 | 583.2 |
| TS | 6.752 | 1.096 | -232.7 | 522.2 |
| vdW-DF | 7.121 | 1.061 | -413.6 | 366.9 |
| vdW-DF2 | 7.064 | 0.974 | -450.8 | 381.6 |
| vdW-DF-cx | 6.514 | 1.128 | -90.5 | 635.6 |
| vdW-DF-ob86 | 6.599 | 1.115 | -149.0 | 589.4 |
| vdW-DF3-opt1 | 6.535 | 1.132 | -100.6 | 622.7 |
| vdW-DF3-opt2 | 6.579 | 1.114 | -138.8 | 600.2 |
| rVV10 | 6.658 | 1.009 | -251.9 | 565.1 |

TABLE I. Equilibrium interlayer distance $d_0$, energy gap $\Delta E$, energy differences of the VB between $\Gamma$ and $K$ points, $\Delta_{\Gamma K}$, and between two highest occupied bands at the $\Gamma$ point, $\Delta_{\Gamma_0 \Gamma_{-1}}$, obtained for different vdW-corrected methods.

The values of $d_0$ reported in other works are comparable to our results [25], including RPA calculations [26].

### C. Effect of deposition and encapsulation on untwisted $WSe_2$

Once we established the computational details, we focus on the effect of capping layers and consider two hexagonal monolayers – AlN and GaN – which can serve as substrates or encapsulations. We construct the initial geometries by assuming the in-plane lattice constant to be the same for all layers, $a = 3.288$ Å, while the values of interlayer distances correspond to their respective bulk structures. We point out that this simplified approach is not suitable for commonly used $h$-BN layers as it gives an unrealistically strained (by $\sim 30\%$) lattice constant. In Fig. 2, we present the $\Delta_{\Gamma K}$ dependence on the interlayer distance $d$ for parallel and antiparallel commensurate stackings. Overall, $\Delta_{\Gamma K}$ decreases linearly with $d_0$ and we observe only a small ($\sim$ 10 meV) difference in a slope of linear fit for deposited and encapsulated structures.

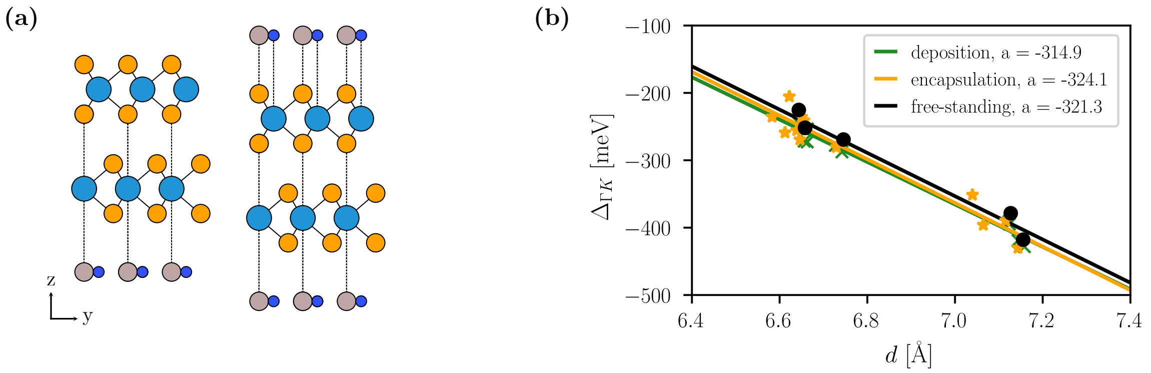


FIG. 2. (a) Side view of $WSe_2$ bilayers in a XM parallel configuration deposited and encapsulated with GaN layers. (b) $\Delta_{\Gamma K}$ as a function of an optimal interlayer distance for six high-symmetric stackings, free-standing and capped. The estimates of the regression slope (in meV/Å) are provided in the legend.

### D. Extraction of pressure

To simulate the experimental situation where a uniaxial vertical pressure $P$ is applied to the system, relaxations for different values of the interlayer distance $d$ were performed. In these calculations also the in-plane lattice parameter $a$ is optimized until the in-plane components of the stress tensor fall below 0.01 kbar. The corresponding pressure is then obtained from the calculated out-of-plane stress component by properly correcting by a geometrical factor $c/(2d)$ to account for the fact that the physical volume of the system is not given by the size of the orthogonal lattice parameter but by roughly $2d$ (due to the added vacuum region). We checked that this approach gives essentially the same results as taking the derivative of the total energy as a function of the interlayer distance, i.e. $P = -\frac{1}{S}\frac{\partial E(d)}{\partial d}$, where $S$ is the unit cell area at a given $d$.

The relation between the pressure and the interlayer distance can be fitted by the Murnaghan relation

$$P = A(e^{-B(1-d/d_0)} - 1). \tag{1}$$

The resulting fits are shown in Table II.

Using the Murnaghan fit, we can extract find for a wide range of pressure value from 0 to 6 GPa the energies of the top of the valence bands. The results are shown in Fig. 3. This data allows us to extract the moiré potential and phase, following the procedure explained

| stacking | $A$ | $B$ | $d_0$ |
|---|---|---|---|
| $MM_{AP}$ | 1.97675 | -11.2359 | 6.64672 |
| $XX_{AP}$ | 1.61687 | -16.2988 | 7.08049 |
| $XM_{AP}$ | 1.80972 | -15.0477 | 6.58404 |
| $XX_P$ | 1.61846 | -16.2229 | 7.10819 |
| $MX_P$ | 1.79177 | -13.8125 | 6.5791 |
| $XM_P$ | 1.78953 | -13.8244 | 6.57906 |

TABLE II. The Murnaghan fits following Eq. (1) of the six different high-symmetry stackings of untwisted bilayer $WSe_2$.

in the main manuscript, as a function of pressure.

## II. LATTICE RELAXATION OF MOIRÉ SUPERCELLS

We apply the coincidence lattice method [27] to construct rigid commensurate superlattices at twist angles above 3°. To relax the atomic structures of twisted bilayers, we performed the classical force field simulations with the LAMMPS package [28]. For intralayer interactions, we used the Stillinger-Weber (SW) potential [29], whereas for the interlayer interactions, we employed the Kolmogorov-Crespi registry-dependent potential [30] with a parametrization according to Ref. 31. The energy minimization was done with fire algorithm and a convergence criterion on the forces of $10^{-8}$ eV/Å.

For each of the supercell, we identify three high-symmetry stackings, which centers are located at fractions of the superlattice vectors $n \cdot (a_1 + a_2)/3$, $n = 0, 1, 2$. Then, we find the W atoms within the radius $R = 6$ Å around each center and compute average in-plane and interlayer distances. We list the results in Tables III and IV.

Even though the interlayer distance can vary up to 0.3 Å throughout one moiré unit cell, it follows the predicted interlayer distances from the untwisted bilayers: the regions with the largest $d$ corresponds to the local XX stacking orders. Se-Se bond lengths (within one layer) change up to 0.2 Å, being the longest in-between commensurate regions. W-Se bonds in both layers do not change significantly over the moiré unit cell ($\sim$ 0.03 Å). Overall, these observations are fully consistent with our DFT results for commensurate unit cells.

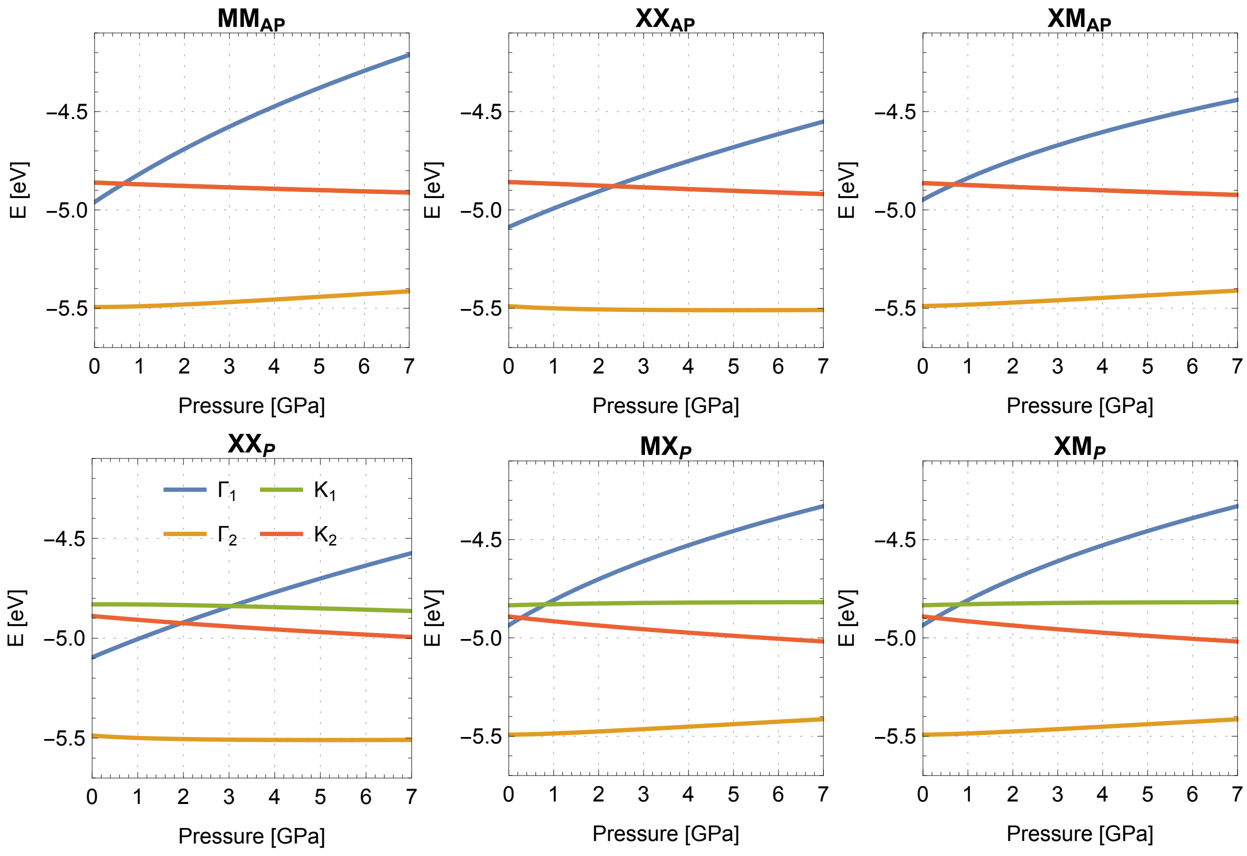


FIG. 3. The energies of the top two valence bands at the $\Gamma$ and $K$ point, for the six different stackings of untwisted bilayers, as a function of pressure. Here $\Gamma_1$ refers to the highest spin-degenerate band at $\Gamma$, and $\Gamma_2$ the second valence band. The state at $K_1$ is the spin-nondegenerate top of the valence band. Note that for antiparallel stackings, the energy of $K_1$ is the same as $K_2$.

## III. THE MOIRÉ ELECTRONIC STRUCTURE

Upon extracting the moiré potential amplitude and phase, we use the continuum model developed by Ref. [32] to calculate the effective flat band structure. The precise model is slightly different for $K$ and $\Gamma$ valleys.

In both cases, given a twist angle $\theta$, the reciprocal moiré lattice vectors $\mathbf{g}_j$ are given by rotating the first moiré lattice vector

$$\mathbf{g}_1 = \left( \frac{4\pi}{\sqrt{3}a_0}\theta, 0 \right) \tag{2}$$

where $a_0 = 3.32$ Å is the monolayer lattice constant of $WSe_2$, and $\theta$ is in radians.

We calculate the band structure using a set of 91 copies of the mini-Brillouin zone.

| | XX | | XM | | MX | |
|---|---|---|---|---|---|---|
| twist [°] | $a$ [Å] | $d$ [Å] | $a$ [Å] | $d$ [Å] | $a$ [Å] | $d$ [Å] |
| 2.5 | 3.308 | 7.186 | 3.279 | 6.69 | 3.279 | 6.69 |
| 2.7 | 3.307 | 7.187 | 3.278 | 6.689 | 3.278 | 6.689 |
| 3.2 | 3.305 | 7.26 | 3.274 | 6.685 | 3.274 | 6.685 |
| 4.4 | 3.304 | 7.275 | 3.266 | 6.68 | 3.265 | 6.68 |
| 5.1 | 3.305 | 7.245 | 3.263 | 6.682 | 3.261 | 6.682 |
| 6.0 | 3.308 | 7.231 | 3.26 | 6.692 | 3.257 | 6.692 |

TABLE III. In-plane and interlayer distances of local commensurate stackings in twisted parallel $WSe_2$ bilayers

| | MM | | XX | | XM (2H) | |
|---|---|---|---|---|---|---|
| twist [°] | $a$ [Å] | $d$ [Å] | $a$ [Å] | $d$ [Å] | $a$ [Å] | $d$ [Å] |
| 2.5 | 3.299 | 6.879 | 3.283 | 7.13 | 3.283 | 6.679 |
| 2.7 | 3.302 | 6.878 | 3.283 | 7.129 | 3.281 | 6.677 |
| 3.2 | 3.303 | 6.878 | 3.286 | 7.129 | 3.279 | 6.67 |
| 4.4 | 3.302 | 6.878 | 3.289 | 7.113 | 3.271 | 6.66 |
| 5.1 | 3.308 | 6.88 | 3.291 | 7.103 | 3.268 | 6.662 |
| 6.0 | 3.259 | 6.863 | 3.293 | 7.077 | 3.265 | 6.678 |

TABLE IV. In-plane and interlayer distances of local commensurate stackings in twisted antiparallel $WSe_2$ bilayers

### A. Γ valley

In the Γ valley, the bands of a monolayer are spin-degenerate and approximated by a parabolic dispersion $-\frac{k^2}{2m_\Gamma}$ where the effective mass is given by $m_\Gamma = 1.68$. The effective model for the moiré flat bands is then given by a $2 \times 2$ matrix in layer-space:

$$H = \begin{bmatrix} -\frac{\hbar^2\mathbf{k}^2}{2m_\Gamma} + V_1 & t_\perp(\mathbf{k}) \\ t_\perp(\mathbf{k}) & \frac{\hbar^2\mathbf{k}^2}{2_\Gamma} + V_2 \end{bmatrix}$$

$$V_{1,2} = 2V_0 \sum_{j=1}^{3} \cos(\mathbf{g}_j \cdot \mathbf{r} \pm \phi) \tag{3}$$

where $V_0$ and $\phi$ depend on the pressure, stacking (parallel/antiparallel) and twist angle. The interlayer hopping $t_\perp(\mathbf{k})$ has a momentum-dependence extracted from first principle calculations of Ref. [33], and an amplitude that is set by the pressure, stacking and twist angle.

Note that the model we used here is the same (at zero pressure) as the one that was used in Ref. [33] to fit the ARPES experimental data. Similar continuum theoretical models of the $\Gamma$ states are developed in Refs. [34, 35].

### B. $K$ valley

At the $K$ valley, we also start with a monolayer description using a parabolic band, with different effective mass $m_K = 0.45$. The main difference is that the bands are spin-nondegenerate, and the top of the valence band is at the $K$-points in both layers which are *not* at the same momenta. We denote $K_t$ the $K$ point of the top layer, and $K_b$ the $K$ point of the bottom layer. The moiré flat bands are now given by

$$H = \begin{bmatrix} -\frac{\hbar^2(\mathbf{k}-\mathbf{K}_t)^2}{2m_K} + V_t & w \\ w^* & \frac{\hbar^2(\mathbf{k}-\mathbf{K}_b)^2}{2m_K} + V_b \end{bmatrix}$$

$$V_{t,b} = 2V_0 \sum_{j=1}^{3} \cos(\mathbf{g}_j \cdot \mathbf{r} + \phi_{t,b}) \tag{4}$$

The moiré phase is $\phi_t = \phi_b$ for the antiparallel stacking and $\phi_t = -\phi_b$ (like in the $\Gamma$ valley) for the parallel stacking structures. Again, each parameter is dependent on the twist angle, pressure and stacking.

Similar continuum theoretical models of the $K$ states are developed in Refs. [32, 36, 37].

## IV. CALCULATION OF THE COULOMB INTERACTION

### A. Constrained RPA

Using the constrained Random Phase Approximation (cRPA) [38] based on ab initio calculations [39, 40], we calculate the Coulomb interactions $U$ for the six bilayer stackings of $WSe_2$ at different pressures. The partially screened Coulomb interaction matrix elements $U_{ijkl}$ are evaluated within the relevant Wannier orbital basis sets and using Kaltak's projector method as recently implemented in VASP [41]. In Fig. 4(a) and (b) are shown $U_{ij} = U_{iijj}$ for $d_{z^2}$ and $d_{xy}$ (similar for $d_{x2-y2}$) orbitals as a function of the distance $r_{ij}$ between sites $i$ and $j$ and pressure $P$. Next, we map the discretized $U_{ij}$ to a continuous model $U(r = r_i - r_j)$ using the image-charge model [42–45] for the potential within a dielectric slab of height $H$:

$$U(\varepsilon_m, \delta, \varepsilon_0, H, r) = \frac{e}{\varepsilon_m}\left[\frac{1}{\sqrt{r^2+\delta}^2} + 2\sum_{n=1}^{\infty}\frac{1}{\sqrt{r^2+\delta^2+(nH)^2}}\left(\frac{\varepsilon_m-\varepsilon_0}{\varepsilon_m+\varepsilon_0}\right)^n\right], \tag{5}$$

where $e$ is the elementary charge, $\delta$ is the parameter allowing to fit the on-site potential $U_{ii} = U(r = 0)$, $\epsilon_m$ is the dielectric constant of the slab, and $\epsilon_0$ represents an additional ab initio screening due to the finite supercell height. Note, in reality, this $\epsilon_0$ can be viewed as the substrate screening; it can be tuned and, therefore, is not a weakness but a feature of our calculations.

We fit $U_{ij}$ individually for each bilayer stacking. Fitted parameters are only $\epsilon_m$ and $\delta$, while $H = 2d$ (twice the interlayer distance, see Table II) and $\epsilon_0 = \epsilon(q = 0)$ are fixed. Here, a slight difference (less than 4%) between the local and nearest neighbour (in and out-of-plane) $U_{ij}$ for different bilayer stackings allows us to use parameters of the fitting function $U$ averaged over six structures for each orbital type and pressure $P$, see Figs. 4(a) and (b). Also, as shown in Fig. 4(c), the values of $U(r)$ only at $r = 0$ slightly become larger with the pressure, indicating that pressure has a negligible effect on Coulomb interaction in the bilayer of $WSe_2$.

### B. Moiré Hubbard U

The continuum model flat bands (see Sec. III) are Wannierized using a 7 momentum-point (the six $K$ points and the $\Gamma$ point) average of the Bloch wavefunctions, where the phase of each Bloch wavefunction is chosen such that the overlap with a Gaussian orbital,

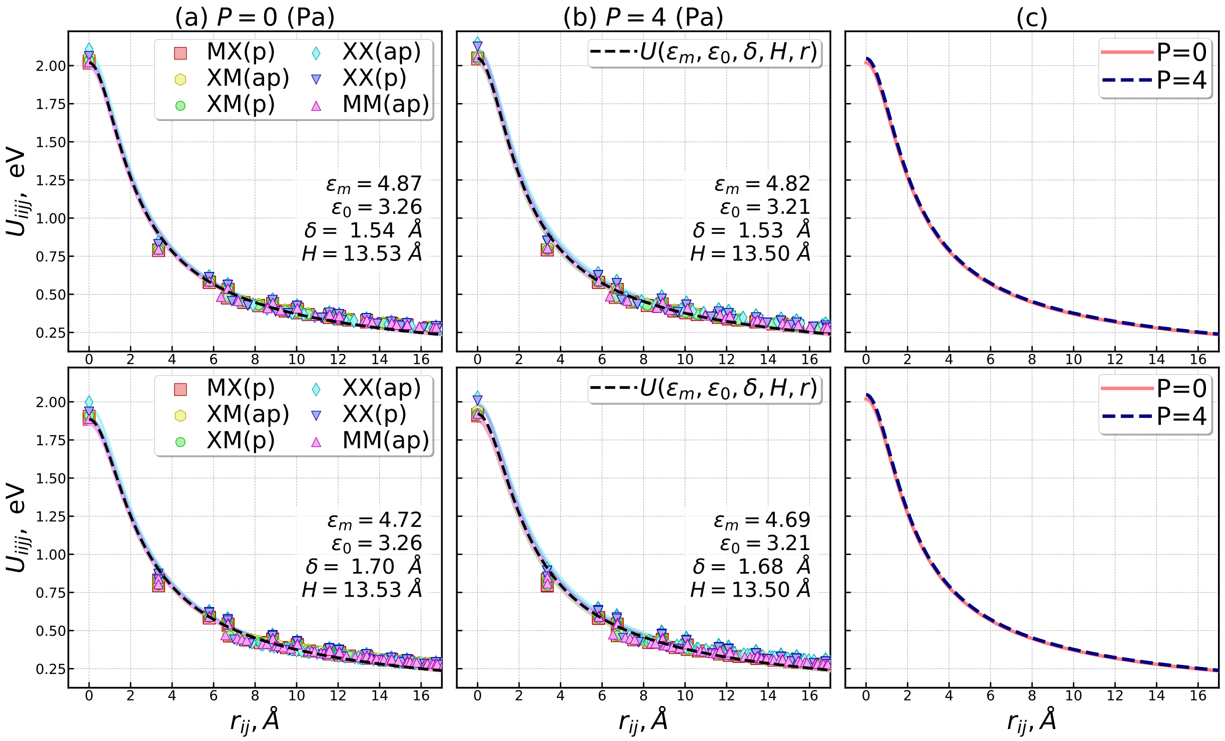


FIG. 4. Coulomb interactions $U_{ij}$ as a function of distance calculated using the constrained Random Phase Approximation. (a) and (b) show results for $P = 0$ and $P = 4$ GPa, respectively for all six bilayer stackings of WSe2. Upper and lower panels shows $U_{ij}$ for $d_{z^2}$ and $d_{xy}$ (similar for $d_{x2-y2}$) orbitals, respectively. Dashed black lines in (a) and (b) represent fits $U(r) = U(\epsilon_m, \epsilon_0, \delta, H, r)$ with averaged parameters for all six bilayer stackings. Plots in (c) show fitted $U(r)$ for two different pressures.

centered at the position where the local density of states is highest, is maximized. The result is a *continuous envelope* for the Wannier functions, depending on the twist angle, pressure and stacking.

We then project and normalize this Wannier envelope on the twisted lattice (see Fig. 5), so that each W site has a weight $w_r$. For the $\Gamma$ valley states, the corresponding local orbitals are $d_{z^2}$ orbitals, whereas for the $K$ valley they are $d_{xy}/d_{x^2-y^2}$ orbitals. The moiré Hubbard $U$ is calculated as a double sum over all $W$ sites $r, r'$

$$U_{\text{moiré}} = \sum_{rr'} U(r_i - r_j)|w_r|^2|w_{r'}|^2 \tag{6}$$

where $U(r)$ is the continuous fit of Eq. (5). The resulting values of the moiré Hubbard $U$ are shown in Table V (for zero pressure) and Table VI (at $P = 4$ GPa).

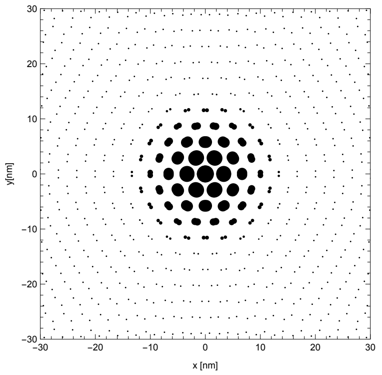


FIG. 5. A visualization of the moiré Wannier orbital, for twist angle $\theta = 3^\circ$ in the $\Gamma$ valley at zero pressure and antiparallel stacking. This Wannier orbital has a Gaussian envelope centered at the $\mathrm{MM_{AP}}$ stacking, with width $\sigma = 9.47$ Å. Size of the dots correspond with the weight-squared of the Wannier orbital.

Note that we ignore the Hubbard $U$ in the $K$ valley of the antiparallel stackings, as there the interlayer coupling is vanishing due to symmetry, which makes that the moiré bands are nothing but uncorrelated backfolded monolayer bands.

## V. MEAN FIELD THEORY

### A. Noninteracting dispersions

We study the triangular lattice models (for the antiparallel $\Gamma$ valley and parallel $K$ valley) and honeycomb lattice model (for the parallel $\Gamma$ valley) with onsite Hubbard moiré $U$ using standard self-consistent Hartree-Fock mean field theory.

For a given moiré length $a_M$, the relevant non-interacting energy dispersions are as follows. Parallel, $K$ valley:

$$\begin{aligned}\epsilon_{\mathbf{k}} &= 2t\left(2\cos\left(\frac{1}{2}\sqrt{3}a_M k_x\right)\cos\left(\frac{a_M k_y}{2}\right)+\cos(a_M k_y)\right)\\ &\quad +2t'\left(\cos\left(\frac{1}{2}a_M\left(\sqrt{3}k_x+3k_y\right)\right)+\cos\left(\frac{1}{2}a_M\left(\sqrt{3}k_x-3k_y\right)\right)+\cos\left(\sqrt{3}a_M k_x\right)\right) \qquad (7)\end{aligned}$$

Parallel, $\Gamma$ valley:

$$\gamma_{\mathbf{k}} = e^{-\frac{1}{6}ia_M\left(\sqrt{3}k_x-3k_y\right)}+e^{-\frac{ia_M\left(k_x+\sqrt{3}k_y\right)}{2\sqrt{3}}}+e^{\frac{ia_M k_x}{\sqrt{3}}} \qquad (8)$$

$$\epsilon_{\mathbf{k}} = \pm t|\gamma_{\mathbf{k}}|+2t'\left(2\cos\left(\frac{1}{2}\sqrt{3}a_M k_x\right)\cos\left(\frac{a_M k_y}{2}\right)+\cos(a_M k_y)\right). \qquad (9)$$

| twist angle $\theta$ | stacking | valley | Wannier size [Å] | $U$ [eV] |
|---|---|---|---|---|
| 3. | P | K | 20.4738 | 0.0505906 |
| 3. | P | Γ | 8.35895 | 0.170488 |
| 3. | AP | Γ | 9.4769 | 0.132196 |
| 3.5 | P | K | 17.6316 | 0.0605974 |
| 3.5 | P | Γ | 7.42437 | 0.178993 |
| 3.5 | AP | Γ | 8.34679 | 0.153824 |
| 4. | P | K | 15.4753 | 0.0715005 |
| 4. | P | Γ | 6.67434 | 0.198676 |
| 4. | AP | Γ | 7.44412 | 0.175617 |
| 4.5 | P | K | 13.785 | 0.0829169 |
| 4.5 | P | Γ | 6.05879 | 0.2205 |
| 4.5 | AP | Γ | 6.70954 | 0.19734 |
| 5. | P | K | 12.4254 | 0.0946276 |
| 5. | P | Γ | 5.54479 | 0.24209 |
| 5. | AP | Γ | 6.10175 | 0.218832 |

TABLE V. The value of moiré Hubbard $U$ for various stackings, valleys and twist angles. For completeness we include the size of the Wannier orbital. These results are at zero pressure.

Antiparallel, $K/K'$ valley, with $\phi = \pm\frac{2\pi}{3}$ depending on the spin/valley:

$$\begin{aligned}\epsilon_{\mathbf{k}} \;=\; & 2t\left(\cos\left(\frac{1}{2}\left(\sqrt{3}a_M k_x + a_M k_y + 2\phi\right)\right) + \cos\left(\frac{1}{2}\left(\sqrt{3}a_M k_x - a_M k_y - 2\phi\right)\right) + \cos(a_M k_y - \phi)\right) \\ & +2t'\left(\cos\left(\frac{1}{2}a_M\left(\sqrt{3}k_x + 3k_y\right)\right) + \cos\left(\frac{1}{2}a_M\left(\sqrt{3}k_x - 3k_y\right)\right) + \cos\left(\sqrt{3}a_M k_x\right)\right). \qquad (10)\end{aligned}$$

Finally, antiparallel, Γ valley has the same dispersion as the parallel $K$ valley of Eq. (7).

The momenta $k_x, k_y$ are chosen in the mini-Brillouin zone. The parameters $t, t'$ for each model are pressure and twist-angle dependent. The Γ state energies are shifted by $\Delta_{\Gamma K}$. The relevant bandstructures for selected pressures is shown in Fig. 6.

| twist angle $\theta$ | stacking | valley | Wannier size [Å] | $U$ [eV] |
|---|---|---|---|---|
| 3. | P | K | 24.0269 | 0.0427344 |
| 3. | P | Γ | 8.19165 | 0.175309 |
| 3. | AP | Γ | 8.24244 | 0.157326 |
| 3.5 | P | K | 19.7695 | 0.0528956 |
| 3.5 | P | Γ | 7.29048 | 0.18395 |
| 3.5 | AP | Γ | 7.39972 | 0.178258 |
| 4. | P | K | 16.8684 | 0.0643236 |
| 4. | P | Γ | 6.56525 | 0.204012 |
| 4. | AP | Γ | 6.71228 | 0.198925 |
| 4.5 | P | K | 14.7458 | 0.0763961 |
| 4.5 | P | Γ | 5.96826 | 0.226062 |
| 4.5 | AP | Γ | 6.13574 | 0.219446 |
| 5. | P | K | 13.117 | 0.0887571 |
| 5. | P | Γ | 5.46827 | 0.24786 |
| 5. | AP | Γ | 5.64379 | 0.23983 |

TABLE VI. The value of moiré Hubbard $U$ for various stackings, valleys and twist angles. For completeness we include the size of the Wannier orbital. These results are at pressure $P = 4$ GPa.

### B. Numerical procedure

The numerical procedure is as follows. Given pressure, twist angle, and stacking, we have a specific set of hopping parameters, valley offset and interaction strengths $U$. We additionally vary the electronic density, as measured by the number of *holes* $\nu$ per moiré unit cell with respect to the top of the valence band. We start with an ansatz for the onsite self-energy $\Sigma_{\sigma\sigma'}(i)$, which in general can mix the spin as well and depends on the site $i$ within the supercell. For triangular lattice models we use a three-sublattice supercell (extended over three moiré unit cells) that allows for 120 degree antiferromagnetic order. For the honeycomb lattice there are already two lattice sites in the unit cell, so the supercell is just one moiré cell. Given the onsite self-energy ansatz, we calculate all the electronic energies on a $48 \times 48$ momentum grid. We then find the chemical potential $\mu$ such that it

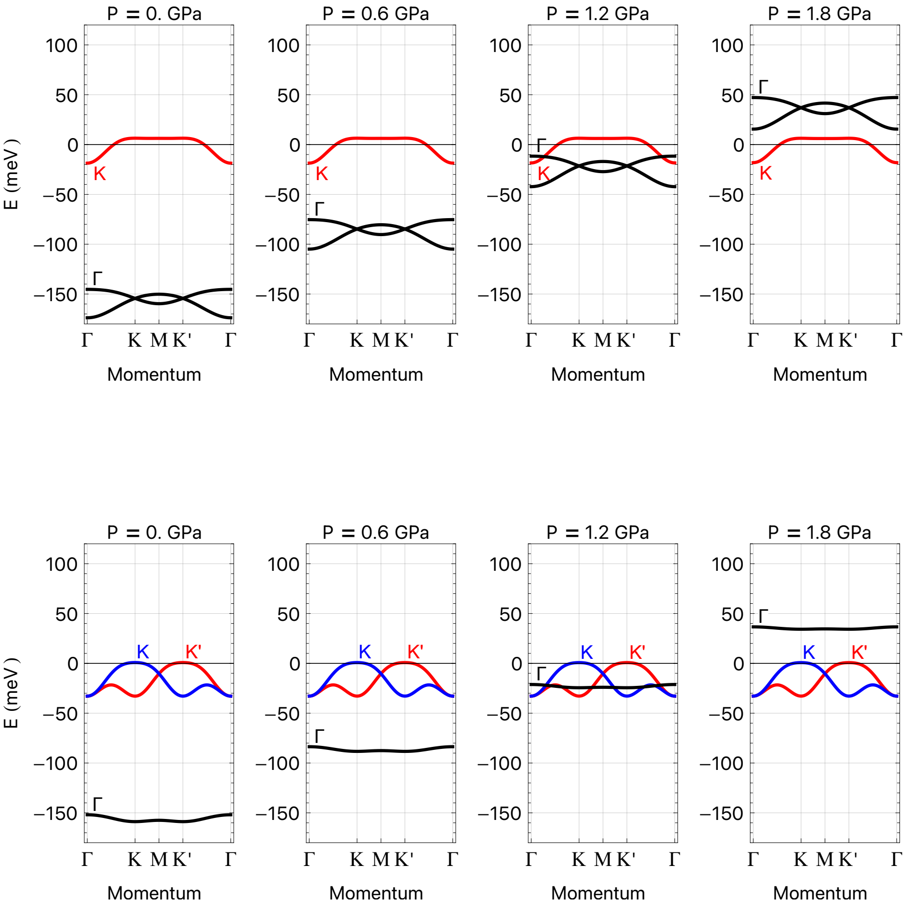


FIG. 6. **Top:** The non-interacting bandstructures used in the mean field theory for the **parallel** stacking case for selected pressures. The twist angle is $\theta = 3°$. **Bottom:** The non-interacting bandstructures used in the mean field theory for the **antiparallel** stacking case for selected pressures.

gives the desired hole density $\nu$. We then calculate the expectation value of the single particle density matrix $\rho_{\sigma\sigma'} = \langle c^{\dagger}_{i\sigma} c_{i\sigma'} \rangle$ for each site $i$ inside our supercell. The new Hartree-Fock self-energy on each site is given by

$$\Sigma^{H}_{\sigma\sigma} = U\rho_{\overline{\sigma}\overline{\sigma}}, \tag{11}$$

$$\Sigma^{F}_{\sigma\overline{\sigma}} = -U\rho_{\overline{\sigma}\sigma}, \tag{12}$$

where $\sigma$ refers to the spin, and $\overline{\sigma} = -\sigma$ is the opposite spin. This procedure is repeated until self-consistency is achieved and a new iteration does not change the self-energy. We

compare different converged results by their total zero-temperature mean field energy

$$E = \mu N - U \sum_i (\rho_{\uparrow\uparrow}\rho_{\downarrow\downarrow} - \rho_{\uparrow\downarrow}\rho_{\downarrow\uparrow}) + \frac{1}{N_k} \sum_{k,n} (\epsilon_{k,n} - \mu) n_F(\epsilon_k - \mu) \tag{13}$$

where $N$ is the total number of particles per supercell, $N_k$ the number of momentum points, $\epsilon_{k,n}$ are the mean field single particle energies as a function of momentum $k$ and band $n$, $n_F$ is the Fermi-Dirac distribution at zero $T$.

The resulting converged solution with the lowest energy is then "measured" for its occupation in each valley and magnetic order in each valley. We also calculate the density of states (based on the single particle energies $\epsilon_{k,n}$). The raw results as a function of a range of densities and pressure are shown in Fig. 7 for the antiparallel stacking and in Fig. 8 for the parallel stacking. These are used to construct the phase diagram show in the main text.

---


[1] P. Giannozzi, S. Baroni, N. Bonini, M. Calandra, R. Car, C. Cavazzoni, D. Ceresoli, G. L. Chiarotti, M. Cococcioni, I. Dabo, A. D. Corso, S. d. Gironcoli, S. Fabris, G. Fratesi, R. Gebauer, U. Gerstmann, C. Gougoussis, A. Kokalj, M. Lazzeri, L. Martin-Samos, N. Marzari, F. Mauri, R. Mazzarello, S. Paolini, A. Pasquarello, L. Paulatto, C. Sbraccia, S. Scandolo, G. Sclauzero, A. P. Seitsonen, A. Smogunov, P. Umari, and R. M. Wentzcovitch, QUANTUM ESPRESSO: a modular and open-source software project for quantum simulations of materials, Journal of Physics-Condensed Matter **21**, 395502 (2009).

[2] P. Giannozzi, O. Andreussi, T. Brumme, O. Bunau, M. B. Nardelli, M. Calandra, R. Car, C. Cavazzoni, D. Ceresoli, M. Cococcioni, N. Colonna, I. Carnimeo, A. D. Corso, S. d. Gironcoli, P. Delugas, R. A. J. DiStasio, A. Ferretti, A. Floris, G. Fratesi, G. Fugallo, R. Gebauer, U. Gerstmann, F. Giustino, T. Gorni, J. Jia, M. Kawamura, H.-Y. Ko, A. Kokalj, E. Kucukbenli, M. Lazzeri, M. Marsili, N. Marzari, F. Mauri, N. L. Nguyen, H.-V. Nguyen, A. Otero-de-la Roza, L. Paulatto, S. Poncé, D. Rocca, R. Sabatini, B. Santra, M. Schlipf, A. P. Seitsonen, A. Smogunov, I. Timrov, T. Thonhauser, P. Umari, N. Vast, X. Wu, and S. Baroni, Advanced capabilities for materials modelling with Quantum ESPRESSO, Journal of Physics-Condensed Matter **29**, 465901 (2017).

[3] P. Giannozzi, O. Baseggio, P. Bonfà, D. Brunato, R. Car, I. Carnimeo, C. Cavazzoni, S. d. Gironcoli, P. Delugas, F. F. Ruffino, A. Ferretti, N. Marzari, I. Timrov, A. Urru, and S. Baroni,

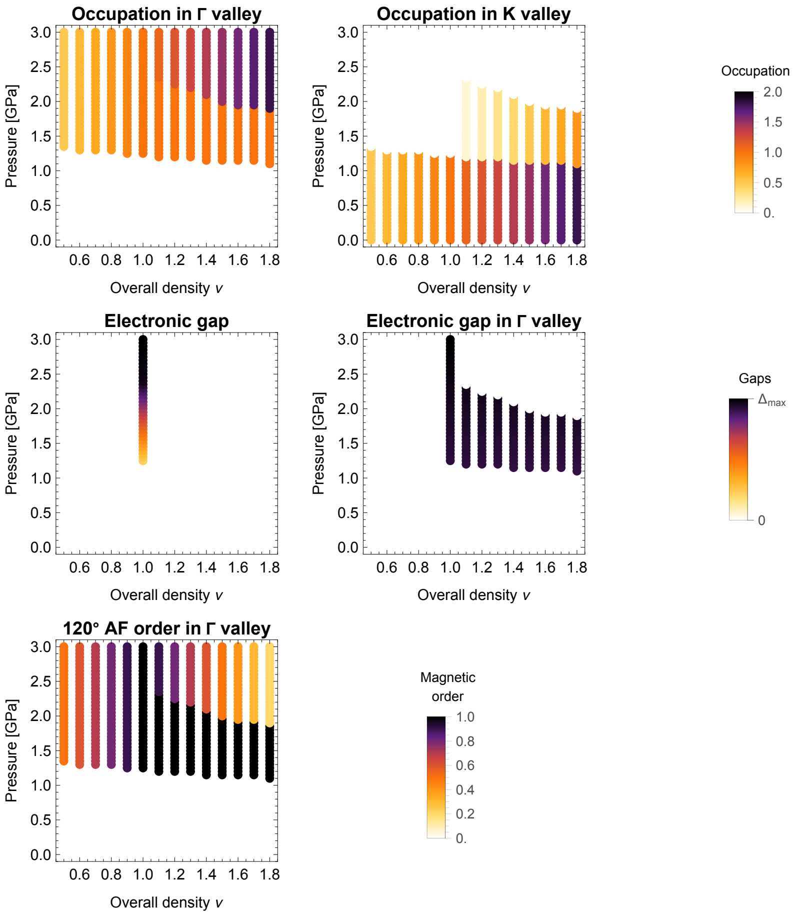


FIG. 7. Mean field theory results for antiparallel stacking at $\theta = 3^\circ$ twist angle and $\epsilon_0 = 30$, showing the valley occupation (top row), electronic gap (middle row) and the magnetic order (bottom figure).

Quantum ESPRESSO toward the exascale, The Journal of Chemical Physics **152**, 154105 (2020), 2104.10502.

[4] M. v. Setten, M. Giantomassi, E. Bousquet, M. Verstraete, D. Hamann, X. Gonze, and G.-M. Rignanese, The PseudoDojo: Training and grading a 85 element optimized norm-conserving pseudopotential table, Computer Physics Communications **226**, 39 (2018), 1710.10138.

[5] C. A. Rozzi, D. Varsano, A. Marini, E. K. U. Gross, and A. Rubio, Exact coulomb cutoff technique for supercell calculations, Phys. Rev. B **73**, 205119 (2006).

[6] T. Sohier, M. Calandra, and F. Mauri, Density functional perturbation theory for gated two-dimensional heterostructures: Theoretical developments and application to flexural phonons in graphene, Phys. Rev. B **96**, 075448 (2017).

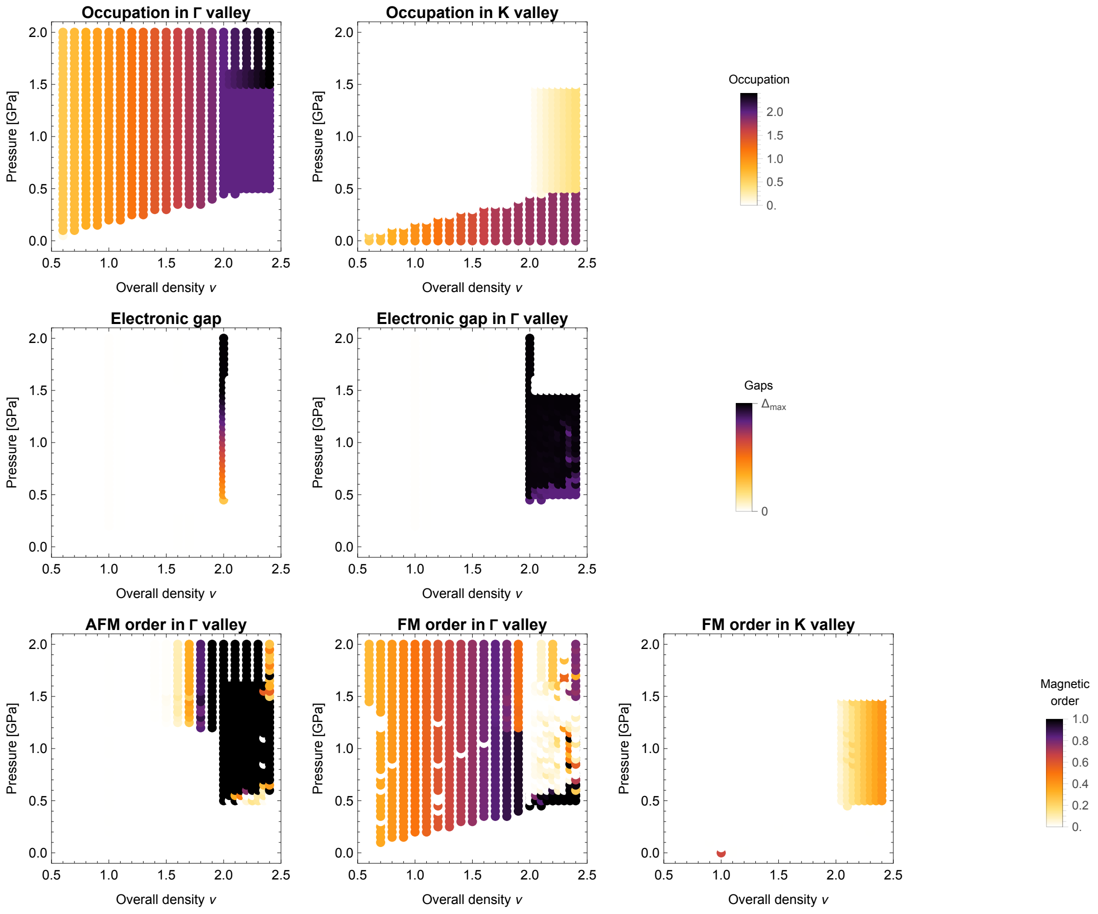


FIG. 8. Mean field theory results for parallel stacking at $\theta = 3^\circ$ twist angle and $\epsilon_0 = 30$, showing the valley occupation (top row), electronic gap (middle row) and the magnetic order (bottom row).

[7] O. A. Vydrov and T. Van Voorhis, Nonlocal van der Waals density functional: The simpler the better, The Journal of Chemical Physics **133**, 244103 (2010).

[8] R. Sabatini, T. Gorni, and S. d. Gironcoli, Nonlocal van der Waals density functional made simple and efficient, Physical Review B **87**, 041108 (2013).

[9] A. H. Larsen, J. J. Mortensen, J. Blomqvist, I. E. Castelli, R. Christensen, M. Dułak, J. Friis, M. N. Groves, B. Hammer, C. Hargus, E. D. Hermes, P. C. Jennings, P. B. Jensen, J. Kermode, J. R. Kitchin, E. L. Kolsbjerg, J. Kubal, K. Kaasbjerg, S. Lysgaard, J. B. Maronsson, T. Maxson, T. Olsen, L. Pastewka, A. Peterson, C. Rostgaard, J. Schiøtz, O. Schütt, M. Strange, K. S. Thygesen, T. Vegge, L. Vilhelmsen, M. Walter, Z. Zeng, and K. W. Jacobsen, The atomic simulation environment—a Python library for working with atoms, Journal of Physics: Condensed Matter **29**, 273002 (2017).

[10] R. Coehoorn, C. Haas, J. Dijkstra, C. J. F. Flipse, R. A. d. Groot, and A. Wold, Electronic structure of MoSe2, MoS2, and WSe2. I. Band-structure calculations and photoelectron spectroscopy, Physical Review B **35**, 6195 (1987).

[11] S. Grimme, Semiempirical GGA-type density functional constructed with a long-range dispersion correction, Journal of Computational Chemistry **27**, 1787 (2006).

[12] V. Barone, M. Casarin, D. Forrer, M. Pavone, M. Sambi, and A. Vittadini, Role and effective treatment of dispersive forces in materials: Polyethylene and graphite crystals as test cases, Journal of Computational Chemistry **30**, 934 (2009).

[13] S. Grimme, J. Antony, S. Ehrlich, and H. Krieg, A consistent and accurate ab initio parametrization of density functional dispersion correction (DFT-D) for the 94 elements H-Pu, The Journal of Chemical Physics **132**, 154104 (2010).

[14] A. Tkatchenko and M. Scheffler, Accurate Molecular Van Der Waals Interactions from Ground-State Electron Density and Free-Atom Reference Data, Physical Review Letters **102**, 073005 (2008).

[15] M. Dion, H. Rydberg, E. Schröder, D. C. Langreth, and B. I. Lundqvist, Van der Waals Density Functional for General Geometries, Physical Review Letters **92**, 246401 (2004), cond-mat/0402105.

[16] T. Thonhauser, S. Zuluaga, C. A. Arter, K. Berland, E. Schröder, and P. Hyldgaard, EnglishSpin Signature of Nonlocal Correlation Binding in Metal-Organic Frameworks, Physical Review Letters **115**, 136402 (2015).

[17] K. Lee, D. Murray, L. Kong, B. I. Lundqvist, and D. C. Langreth, Higher-accuracy van der Waals density functional, Physical Review B **82**, 081101 (2010), 1003.5255.

[18] I. Hamada, van der Waals density functional made accurate, Physical Review B **89**, 121103 (2014).

[19] K. Berland and P. Hyldgaard, Exchange functional that tests the robustness of the plasmon description of the van der Waals density functional, Physical Review B **89**, 035412 (2014), 1309.1756.

[20] J. Klimeš, D. R. Bowler, and A. Michaelides, Chemical accuracy for the van der Waals density functional, Journal of Physics: Condensed Matter **22**, 022201 (2010).

[21] J. Klimeš, D. R. Bowler, and A. Michaelides, Van der Waals density functionals applied to solids, Physical Review B **83**, 195131 (2011), 1102.1358.

[22] H. Peng and J. P. Perdew, Rehabilitation of the Perdew-Burke-Ernzerhof generalized gradient approximation for layered materials, Physical Review B **95**, 081105 (2017), 1612.03524.

[23] D. Chakraborty, K. Berland, and T. Thonhauser, Next-Generation Nonlocal van der Waals Density Functional, Journal of Chemical Theory and Computation **16**, 5893 (2020), 2010.10109.

[24] J. Xu, J. Zhang, W. Zhang, and C. Lee, Interlayer Nanoarchitectonics of Two-Dimensional Transition-Metal Dichalcogenides Nanosheets for Energy Storage and Conversion Applications, Advanced Energy Materials **7**, 10.1002/aenm.201700571 (2017).

[25] N. Morales-Durán, J. Wang, G. R. Schleder, M. Angeli, Z. Zhu, E. Kaxiras, C. Repellin, and J. Cano, Pressure-enhanced fractional Chern insulators along a magic line in moiré transition metal dichalcogenides, Physical Review Research **5**, L032022 (2023), 2304.06669.

[26] J. He, K. Hummer, and C. Franchini, Stacking effects on the electronic and optical properties of bilayer transition metal dichalcogenides MoS2, MoSe2, WS2, and WSe2, Physical Review B **89**, 075409 (2014).

[27] D. S. Koda, F. Bechstedt, M. Marques, and L. K. Teles, Coincidence Lattices of 2D Crystals: Heterostructure Predictions and Applications, The Journal of Physical Chemistry C **120**, 10895 (2016).

[28] A. P. Thompson, H. M. Aktulga, R. Berger, D. S. Bolintineanu, W. M. Brown, P. S. Crozier, P. J. i. t. Veld, A. Kohlmeyer, S. G. Moore, T. D. Nguyen, R. Shan, M. J. Stevens, J. Tranchida, C. Trott, and S. J. Plimpton, LAMMPS - a flexible simulation tool for particle-based materials modeling at the atomic, meso, and continuum scales, Computer Physics Communications **271**, 108171 (2022).

[29] J.-W. Jiang and Y.-P. Zhou, Handbook of Stillinger-Weber Potential Parameters for Two-Dimensional Atomic Crystals, arXiv 10.5772/intechopen.71929 (2017), 1704.03147.

[30] A. N. Kolmogorov and V. H. Crespi, Registry-dependent interlayer potential for graphitic systems, Physical Review B **71**, 235415 (2005).

[31] M. H. Naik, I. Maity, P. K. Maiti, and M. Jain, Kolmogorov–Crespi Potential For Multilayer Transition-Metal Dichalcogenides: Capturing Structural Transformations in Moire Superlattices, The Journal of Physical Chemistry C **123**, 9770 (2019).

[32] F. Wu, T. Lovorn, E. Tutuc, I. Martin, and A. H. MacDonald, EnglishTopological Insulators in Twisted Transition Metal Dichalcogenide Homobilayers, Physical Review Letters **122**, 086402

(2019).

[33] G. Gatti, J. Issing, L. Rademaker, F. Margot, T. A. d. Jong, S. J. v. d. Molen, J. Teyssier, T. K. Kim, M. D. Watson, C. Cacho, P. Dudin, J. Avila, K. C. Edwards, P. Paruch, N. Ubrig, I. Gutiérrez-Lezama, A. F. Morpurgo, A. Tamai, and F. Baumberger, Flat Moiré Bands in Twisted Bilayer WSe2, Physical Review Letters **131**, 046401 (2023), 2211.01192.

[34] Y. Zhang, T. Liu, and L. Fu, Electronic structures, charge transfer, and charge order in twisted transition metal dichalcogenide bilayers, Physical Review B **103**, 155142 (2021).

[35] M. Angeli and A. H. MacDonald, valley transition metal dichalcogenide moiré bands, Proceedings of the National Academy of Sciences **118**, e2021826118 (2021), 2008.01735.

[36] T. Devakul, V. Crépel, Y. Zhang, and L. Fu, Magic in twisted transition metal dichalcogenide bilayers, Nature Communications **12**, 6730 (2021), 2106.11954.

[37] H. Pan, F. Wu, and S. D. Sarma, EnglishBand topology, Hubbard model, Heisenberg model, and Dzyaloshinskii-Moriya interaction in twisted bilayer WSe2, Physical Review Research **2**, 033087 (2020).

[38] F. Aryasetiawan, M. Imada, A. Georges, G. Kotliar, S. Biermann, and A. I. Lichtenstein, Frequency-dependent local interactions and low-energy effective models from electronic structure calculations, Phys. Rev. B **70**, 195104 (2004).

[39] G. Kresse and J. Furthmüller, Efficiency of ab-initio total energy calculations for metals and semiconductors using a plane-wave basis set, Comp. Mat. Sci. **6**, 15 (1996).

[40] G. Kresse and J. Furthmüller, Efficient iterative schemes for *ab initio* total-energy calculations using a plane-wave basis set, Phys. Rev. B **54**, 11169 (1996).

[41] M. Kaltak, Merging GW with DMFT (2015), PhD Thesis, University of Vienna (2015).

[42] L. V. Keldysh, Coulomb interaction in thin semiconductor and semimetal films, Sov. J. Exp. Theor. Phys. Lett. **29**, 716 (1979).

[43] Z. Jiang, S. Haas, and M. Rösner, Plasmonic waveguides from coulomb-engineered two-dimensional metals, 2D Materials **8**, 035037 (2021).

[44] D. Jena and A. Konar, Enhancement of carrier mobility in semiconductor nanostructures by dielectric engineering, Phys. Rev. Lett. **98**, 136805 (2007).

[45] A. Emelyanenko and L. Boinovich, On the effect of discrete charges adsorbed at the interface on nonionic liquid film stability: charges in the film, Journal of Physics: Condensed Matter **20**, 494227 (2008).
